# Supplementary material for: Understanding and Mitigating the Threat of Vec2Text to Dense Retrieval Systems
Source: arXiv:2402.12784 source file (2024-07-24)
Supplement: Supplementary file 1 [file appendix.tex]

\section{Prompts used in this study}
